# Supplementary material for: A Geometric VOF Method for Interface Flow Simulations
Source: arXiv:2402.05247 source file (2024-02-07)
Supplement: Supplementary file 1 [file appendix.tex]

\section*{Appendix A: Reconstructed PLIC Interfaces with Various Orientation Schemes}

\setcounter{figure}{0}
